# Supplementary material for: Learning Predictive Representations for Deformable Objects Using Contrastive Estimation
Source: arXiv:2003.05436 source file (2020-03-11)
Supplement: Supplementary file 1 [file appendix.tex]

\section{Appendix}
\subsection{Pointmass Environment}

We also experimented with a toy pointmass environment, where, similar to the rope and cloth environments, the observation is a $64\times 64\times 3$ RGB image. The action is a two-dimensional vector describing the $x,y$ perturbation of the pointmass from its current location. We evaluate our method by performing the same manner of MPC as with the other environments, and compute the $\ell_2$-distance between the achieved and goal locations of the pointmasses. In Table~\ref{table:pointmass}, we show results comparing our method against other baselines, and can see that PlaNet performs competitively with CFM in the task to move the pointmass to the center, but does substantially worse in the case harder task setting when a goal state is randomly chosen, whereas our method maintains its accuracy. This may show that contrastive methods can learn and generalize better with less data compared to existing methods.

\begin{table}[H]
\caption{Evaluation results for the pointmass environments comparing our method against different baselines}
\centering
\begin{tabular}{l|ll}
\hline
                              & \textbf{Center}  & \textbf{Random} \\ \hline
\textbf{Random Policy}        & $0.24$                   & $0.32$          \\
\textbf{Autoencoder}          & $0.16 \pm 0.03$          & $0.22 \pm 0.01$ \\
\textbf{PlaNet}               & $0.05 \pm 0.01$          & $0.20 \pm 0.01$ \\
\textbf{Joint Dynamics Model} & $0.18 \pm 0.11$          & $0.25 \pm 0.13$ \\
\textbf{Visual Forward Model} & $0.36 \pm 0.02$          & $0.36 \pm 0.02$ \\
\textbf{CFM (ours)}           & $\mathbf{0.02 \pm 0.01}$ & $\mathbf{0.05 \pm 0.01}$
\end{tabular}
\label{table:pointmass}
\end{table}
